# Supplementary material for: Efficient and DoS-resistant Consensus for Permissioned Blockchains
Source: arXiv:1808.02252 source file (2020-12-15)
Supplement: Supplementary file 1 [file 10appendix.tex]

% \widowpenalty0
% \clubpenalty0
